# Supplementary material for: What is the stable atomic structure of NiTi austenite?
Source: arXiv:1404.0423 source file (2014-07-14)
Supplement: Supplementary file 1 [file NiTi_Supplement.pdf]

Supplementary Information

# What is the stable atomic structure of NiTi austenite?

Nikolai A. Zarkevich & Duane D. Johnson

**Table S1**. Direct lattice coordinates of the Ni and Ti atoms in a fixed hexagonal (left) and fully relaxed (right) unit cell representing the austenite structure. The lattice translation vectors in the fixed hexagonal cell are *a*=*b*=12.73992 Å and *c*=5.20105 Å; the calculated external pressure is 1.96 kB, with the pressure tensor components of 12.78, 14.88, -21.77, -0.78, -6.94, and -0.61 kB along x, y, z, xy, yz, and zx directions, respectively. Full relaxation at zero pressure changes the lattice constants to *a*=12.88133, *b*=12.94640, and *c*=5.09557 Å and angles between them to $\alpha$=91.81, $\beta$=92.71, and $\gamma$=59.62 degrees. Atomic forces after relaxation are below 0.002 eV/Å.

Ni

| Relaxed atoms in a fixed cell | | | Fully relaxed structure | | |
|---|---|---|---|---|---|
| x | y | z | x | y | z |
| 0.333678 | 0.341113 | 0.508004 | 0.337829 | 0.342878 | 0.512187 |
| 0.309585 | 0.660084 | 0.484136 | 0.301768 | 0.664676 | 0.518077 |
| 0.342001 | 0.965413 | 0.512847 | 0.342549 | 0.964317 | 0.510562 |
| 0.687431 | 0.339773 | 0.504771 | 0.697811 | 0.334402 | 0.476544 |
| 0.666952 | 0.658291 | 0.507769 | 0.661830 | 0.655716 | 0.491982 |
| 0.675650 | 0.012495 | 0.422453 | 0.658357 | 0.035111 | 0.488260 |
| 0.028770 | 0.297928 | 0.565198 | 0.032317 | 0.299752 | 0.549254 |
| 0.968228 | 0.705309 | 0.429831 | 0.964212 | 0.703239 | 0.452787 |
| 0.024984 | 0.982245 | 0.479895 | 0.023165 | -0.001092 | 0.500055 |
| 0.411560 | 0.451748 | 0.186412 | 0.403026 | 0.462438 | 0.202069 |
| 0.466103 | 0.768590 | 0.176552 | 0.453831 | 0.772032 | 0.132730 |
| 0.452224 | 0.133285 | 0.191862 | 0.451507 | 0.138947 | 0.199867 |
| 0.770750 | 0.446233 | 0.171958 | 0.774301 | 0.443514 | 0.159729 |
| 0.774588 | 0.800111 | 0.088773 | 0.778725 | 0.783768 | 0.077646 |
| 0.756907 | 0.141317 | 0.158347 | 0.749859 | 0.132599 | 0.189601 |
| 0.125518 | 0.400881 | 0.253017 | 0.128621 | 0.402078 | 0.246390 |
| 0.120124 | 0.766216 | 0.172793 | 0.107566 | 0.765971 | 0.201956 |
| 0.130872 | 0.104185 | 0.246998 | 0.131148 | 0.108506 | 0.237572 |
| 0.588617 | 0.549530 | 0.827635 | 0.596015 | 0.536277 | 0.798527 |
| 0.550790 | 0.868156 | 0.815681 | 0.547572 | 0.861830 | 0.801530 |
| 0.531671 | 0.248778 | 0.885628 | 0.542695 | 0.232093 | 0.870360 |
| 0.870695 | 0.595822 | 0.778616 | 0.868717 | 0.599471 | 0.760746 |
| 0.871235 | 0.893763 | 0.735497 | 0.863974 | 0.889015 | 0.773218 |
| 0.869885 | 0.239860 | 0.848802 | 0.896367 | 0.230553 | 0.792884 |
| 0.225480 | 0.553699 | 0.836306 | 0.223392 | 0.557016 | 0.841206 |
| 0.227938 | 0.862003 | 0.779532 | 0.240502 | 0.869070 | 0.790520 |
| 0.213064 | 0.217666 | 0.936222 | 0.217235 | 0.219798 | 0.930647 |

**Table S1** (continued).

| Ti | | | | | |
|---|---|---|---|---|---|
| Relaxed atoms in a fixed cell | | | Fully relaxed structure | | |
| x | y | z | x | y | z |
| 0.319316 | 0.334233 | 0.003581 | 0.323385 | 0.336370 | 0.999115 |
| 0.337589 | 0.654791 | 0.001665 | 0.325572 | 0.666628 | 0.028587 |
| 0.341555 | 0.994720 | 0.005527 | 0.345745 | 0.994989 | 0.009847 |
| 0.656530 | 0.346972 | 0.993878 | 0.676154 | 0.329711 | 0.961157 |
| 0.680485 | 0.665821 | 0.018248 | 0.674849 | 0.664286 | 0.004765 |
| 0.653859 | 0.019149 | 0.940124 | 0.656007 | 0.007331 | 0.993422 |
| 0.998944 | 0.320760 | 0.070026 | 0.003898 | 0.322454 | 0.055130 |
| 0.992629 | 0.678817 | 0.944331 | 0.991275 | 0.681360 | 0.951740 |
| 0.000663 | 0.005184 | 0.980643 | 0.000411 | 0.999310 | 0.996190 |
| 0.555543 | 0.550269 | 0.334428 | 0.558518 | 0.535519 | 0.295757 |
| 0.543211 | 0.908096 | 0.308181 | 0.538760 | 0.906045 | 0.299545 |
| 0.553205 | 0.239141 | 0.376531 | 0.552374 | 0.254073 | 0.374297 |
| 0.909975 | 0.556408 | 0.294149 | 0.907839 | 0.555655 | 0.277527 |
| 0.887368 | 0.913075 | 0.237549 | 0.879062 | 0.911210 | 0.281311 |
| 0.899704 | 0.206523 | 0.349511 | 0.900825 | 0.204476 | 0.309541 |
| 0.190817 | 0.553036 | 0.346188 | 0.189134 | 0.554861 | 0.358230 |
| 0.231506 | 0.876581 | 0.289711 | 0.220871 | 0.884805 | 0.290589 |
| 0.250419 | 0.194653 | 0.437918 | 0.252448 | 0.199244 | 0.429748 |
| 0.438774 | 0.457222 | 0.674870 | 0.440391 | 0.464482 | 0.702365 |
| 0.449048 | 0.756793 | 0.672000 | 0.447707 | 0.746007 | 0.632840 |
| 0.456102 | 0.100930 | 0.692560 | 0.459795 | 0.095905 | 0.698791 |
| 0.806534 | 0.443989 | 0.655919 | 0.808998 | 0.444793 | 0.643071 |
| 0.755252 | 0.798125 | 0.585210 | 0.744853 | 0.802631 | 0.572664 |
| 0.782917 | 0.114810 | 0.663690 | 0.791003 | 0.106329 | 0.694934 |
| 0.091137 | 0.441716 | 0.731113 | 0.089360 | 0.446542 | 0.728869 |
| 0.099604 | 0.780105 | 0.660408 | 0.095166 | 0.793951 | 0.684330 |
| 0.119035 | 0.090115 | 0.737077 | 0.127730 | 0.093586 | 0.729299 |
